# Supplementary material for: Constructive Game Logic
Source: arXiv:2002.08523 source file (2020-07-22)
Supplement: Supplementary file 1 [file semantics-appendix.tex]

%TODO: Update for FSCD where everything has differential
We give the precise definitions of differentials $\der{f}$ and solutions $(\solves{sol}{s}{d}{\D{x}=f})$ here.

The differential term $\der{f}$ is definable when $f$ is differentiable.
Not every term $f$ need be differentiable, so we give a \emph{virtual} definition, defining when $\der{f}$ is equal to some term $g$.
If $\der{f}$ does not exist, $\der{f} = g$ is not provable.
We define the (total) derivative as the dot product ($\vdot$) of gradient $\nabla$ with $\D{s},$ which is the vector of values $s\ \D{x}$ assigned to primed variables.
To show that $\nabla$ is the gradient, we define the gradient as a limit, which we express in $(\epsilon,\delta)$ style.
\begin{align*}
  (\der{f}\ s = g\ s) &\equiv
    \lexists[{\xty^{\abs{\D{s}}}}]{\nabla}{}
    (g\ s = \nabla \vdot \D{s}) \kwprod
    \pity{\epsilon}{\reals_+}{\sity{\delta}{\reals_+}{\pity{r}{\sty}{}}}\\
    &\sfun{(\norm{r - s} < \delta )}
        {\abs{f\ r - f\ s - \nabla \vdot (r - s)} \leq \epsilon \norm{r - s}}
\end{align*}
For practical proofs, a library of standard rules for automatic, syntactic differentiation of common arithmetic operations can be proven.

The predicate $(\solves{sol}{s}{d}{\D{x}=f})$ simply employs $\der{sol}$ to say that the solution satisfies the differential equation at every time, and also insures that the solution is compatible with the initial state.
\[\small{(\solves{sol}{s}{d}{\D{x}=f}) \lequiv
\left(
\sprod{(\lget{s}{x} = sol\ 0)}
{\pity{r}{[0,d]}{
   (\der{sol}\ r = f\ (\lset{s}{x}{(sol\ r)}))
}}\right)}\]

The main paper also mentions both active and demonic strategies are constructive, but allow classical opponents.
We give an example here: consider the relationship between active and dormant semantics of $\prandom{x}$.
Angel gives a computable strategy for $x,$ which are countably many.
However, the dormant player does not care how $x$ was determined, and can handle any of the uncountably many values of type $\reals$.
This mirrors the distinction between computable reals (countable) and computable functions over reals (countably many, uncountable domain).
